# Supplementary material for: Hierarchical Micro-Macro Acceleration for Moment Models of Kinetic Equations
Source: arXiv:2209.13356 source file (2022-09-27)
Supplement: Supplementary file 1 [file appendix.tex]

%\appendix
%\section{2D Model equations}
%\label{app:2D_micro}

%\jk{need to include 2D model, either HME from 2D paper or QBME from PI paper or both.}
